# Supplementary material for: Exact Replica Symmetric solution for transverse field Hopfield model under finite Trotter size
Source: arXiv:2411.02012 source file (2025-03-14)
Supplement: Supplementary file 1 [file appendix_secret.tex]

\section{Phase boundary coefficients near $\alpha = 0$} \label{sec:appendix}
In this section, we derive the coefficients $\tau_{\rm R-I, II}(\beta)$, which is given in figure [], which is done by a perturbation analysis on \eqref{eq:hatq_SA}--\eqref{eq:chi_SA} for small $\alpha$. For sake of completeness, we rewrite these equations with the subscript dropped for the order parameters: 
\begin{align}
    \hq &= \frac{\alpha \beta \chi}{1 - \beta \chi}, \\
    \hchi &= \frac{\alpha \beta(q - \chi)}{ (1 - \beta \chi)^2}\\
    m &= \EE_{\mathsf{z}} [ \langle \mu \rangle_{\hq, \zsf} ], \\
    q &= \EE_{\mathsf{z}} [ \langle \mu \rangle_{\hq, \zsf}^2 ], \\
    \chi &= \EE_{\mathsf{z}} [ \langle \mu^2 \rangle_{\hq, \zsf} ] - q,
\end{align}
where $\mu = M^{-1} \sum_{t = 1}^M \sigma_t$, $\zsf \sim \mathcal{N} (0, \hchi)$ and $\av{\cdots}_{\hq, \zsf}$ is the expectation with respect to the canonical distribution with Boltzmann factor 
\begin{equation}
    \exp \Bigg[  \frac{\beta \hq}{2} \mu^2 + (\sqrt{\beta} \zsf + m)  \mu + B \sum_{t = 1}^M \sigma_t \sigma_{t + 1}\Bigg].
\end{equation}
For simplicity, let $\av{\cdots} = \av{\cdots}_{0,0}$, and $\av{\mu^n} = \hat{\mu}_n$. 
To obtain the coefficients for the R-I critical point, we assume that the retrieval state appears as a metastable state when the transverse field is given by $\Gamma = \Gamma^\star(1 - \epsilon)$, where we define $\Gamma^\star = \Gamma_\beta^\star (\beta)$ to lighten notation. Let us expand the equation of states for $q -\chi$, $1 - \beta \chi$ and $m$ for small $\alpha, m, \epsilon$. Noting that for any observable $\mathcal{O}$, the first order expansion for $\hq$ and $\hchi$ is given by 
\begin{gather*}
    \EE_\zsf [ \av{\mathcal{O}}_{\hq, \zsf} ] = \av{\mathcal{O}} + \frac{\beta \hq}{2} ( \av{\mathcal{O}\mu^2} - \av{\mathcal{O}} \hat{\mu}_2  ) \\
    + \frac{\beta \hchi}{2} (  \av{\mathcal{O}\mu^2} - 2 \av{\mathcal{O}\mu} \hat{\mu}_1 + 2 \av{\mathcal{O}} \hat{\mu}_1^2 - \mathcal{O} \hat{\mu}_2  )
    \end{gather*}
    Therefore, up to first leading order, 
    \begin{align*}
        \EE_{\zsf}[ \av{\mu}^2_{\hq, \zsf} ] &= \hat{\mu}_2 + \frac{\beta(\hq + \hchi)}{2} (\hat{\mu}_4 - \hat{\mu}_2^2) ,\\
         \EE_{\zsf}[ \av{\mu}_{\hq, \zsf} ]  &= \hat{\mu}_1 + \frac{\eta\hq}{2} (\hat{\mu}_3 - \hat{\mu}_1 \hat{\mu}_2 ) + \frac{\beta \hchi}{2} (\hat{\mu}_3 - 3 \hat{\mu}_2 \hat{\mu}_1 + 2 \hat{\mu}_1^3),\\
         \EE_{\zsf}[ \av{\mu}_{\hq, \zsf}^2] &= \hat{\mu}_1^2 + \beta \hchi (\hat{\mu}_2 - \hat{\mu}_1^2)^2.
    \end{align*}
    Using these equations, and expanding the moments with respect to $m$ and $\epsilon$ when necessary, the fixed point equations for $m,q,\chi$ satisfy
\begin{align}
   1 - \beta \chi &= - E \epsilon + \frac{3m^2 E}{2} - \frac{\alpha F}{2(1 - \beta \chi)} + \frac{3\alpha(q-\chi) E}{2 (1 - \beta \chi)^2}, \\
   q - \chi &= m^2 + \frac{\alpha (q - \chi) }{ (1 - \beta \chi)^2}\\
   0 &= E\epsilon - \frac{Em^2}{2} + \frac{\alpha F}{2(1-\beta \chi)} - \frac{3\alpha E (q - \chi)}{2 (1 - \beta \chi)^2}
\end{align}
